# Supplementary material for: Sample Efficient Linear Meta-Learning by Alternating Minimization
Source: arXiv:2105.08306 source file (2021-05-18)
Supplement: Supplementary file 1 [file meta_learn_appendix.tex]

\documentclass{article}
\usepackage[utf8]{inputenc}
\usepackage{geometry}
\geometry{ portrait, margin=0.75in} 

\input{notations}

\usepackage{natbib}

\title{Appendix: \metlearntitle}

\begin{document}

\maketitle

\input{rank_one}

\input{rank_r}

\input{technical}

\bibliographystyle{plain}
\bibliography{meta_learn}

\end{document}
